# Supplementary material for: Sickle-cell disease diagnosis support selecting the most appropriate machinelearning method: Towards a general and interpretable approach for cellmorphology analysis from microscopy images
Source: arXiv:2010.04511 source file (2020-10-09)
Supplement: Supplementary file 1 [file appendixD.tex]

%%%%%%%%%%%%% Para hacer pruebas
\appendix
\section{Second experiment: confusion matrices}
\label{appendix-second}

\begin{longtable}{c}

\begin{tabular}{@{}lrrrrrrrrr@{}}
\cmidrule(r){1-4} \cmidrule(lr){5-8} 
\begin{tabular}[c]{@{}l@{}}\textcolor{red}{RF 15} features\\ SDS-score\end{tabular} & c & e & o &   \begin{tabular}[c]{@{}l@{}}\textcolor{red}{RF 15} features\\ F-measure\end{tabular} & c & e & o &\\ \cmidrule(r){1-4} \cmidrule(lr){5-8} 
c & 488 & 7 & 4 &   c & 489 & 7 & 3 &    \\
e & 7 & 194 & 9 &   e & 8 & 194 & 8 & \\
o & 22 & 4 & 74 &   o & 22 & 3 & 75 &  \\ \cmidrule(r){1-4} \cmidrule(lr){5-8} 
\end{tabular}%
%}
%\caption{Fine-tuned DT and RF confusion matrices comparison with all features}
\label{confusion_GB_2}

\\

\begin{tabular}{@{}lrrrrrrrrr@{}}
\cmidrule(r){1-4} \cmidrule(lr){5-8} 
\begin{tabular}[c]{@{}l@{}}\textcolor{red}{DT} 20 features\\ max SDS-score\end{tabular} & c & e & o &   \begin{tabular}[c]{@{}l@{}}\textcolor{red}{DT} 20 features\\ F-measure\end{tabular} & c & e & o &\\ \cmidrule(r){1-4} \cmidrule(lr){5-8} 
c & 483 & 13 & 3 &   c & 483 & 13 & 3 &    \\
e & 8 & 199 & 3 &   e & 8 & 199 & 3 & \\
o & 24 & 9 & 67 &   o & 24 & 9 & 67 &  \\ \cmidrule(r){1-4} \cmidrule(lr){5-8} 
\end{tabular}%
%}
%\caption{Fine-tuned DT and RF confusion matrices comparison with all features}
\label{confusion_rf_2}

\\

\begin{tabular}{@{}lrrrrrrrrr@{}}
\cmidrule(r){1-4} \cmidrule(lr){5-8} 
\begin{tabular}[c]{@{}l@{}}\textcolor{red}{RF} PCA\\ max SDS-score\end{tabular} & c & e & o &   \begin{tabular}[c]{@{}l@{}}\textcolor{red}{RF} PCA\\ max F-measure\end{tabular} & c & e & o &\\ \cmidrule(r){1-4} \cmidrule(lr){5-8} 
c & 485 & 9 & 5 &   c & 485 & 9 & 5 &    \\
e & 14 & 194 & 2 &   e & 14 & 194 & 2 & \\
o & 34 & 12 & 54 &   o & 34 & 12 & 54 &  \\ \cmidrule(r){1-4} \cmidrule(lr){5-8} 
\end{tabular}%

%\caption{Fine-tuned DT and RF confusion matrices comparison with all features}
\label{confusion_gb_3}

\\

\begin{tabular}{@{}lrrrrrrrrr@{}}
\cmidrule(r){1-4} \cmidrule(lr){5-8} 
\begin{tabular}[c]{@{}l@{}}\textcolor{red}{DT} PCA\\ max SDS-score\end{tabular} & c & e & o &   \begin{tabular}[c]{@{}l@{}}\textcolor{red}{DT} PCA\\ max F-measure\end{tabular} & c & e & o &\\ \cmidrule(r){1-4} \cmidrule(lr){5-8} 
c & 483 & 9 & 7 &   c & 483 & 9 & 7 &    \\
e & 25 & 172 & 13 &   e & 25 & 172 & 13 & \\
o & 36 & 11 & 53 &   o & 36 & 11 & 53 &  \\ \cmidrule(r){1-4} \cmidrule(lr){5-8} 
\end{tabular}%

\\

\begin{tabular}{@{}lrrrrrrrrr@{}}
\cmidrule(r){1-4} \cmidrule(lr){5-8} 
\begin{tabular}[c]{@{}l@{}}\textcolor{red}{RF} LDA\\ max SDS-score\end{tabular} & c & e & o &   \begin{tabular}[c]{@{}l@{}}\textcolor{red}{RF} LDA\\ max F-measure\end{tabular} & c & e & o &\\ \cmidrule(r){1-4} \cmidrule(lr){5-8} 
c & 478 & 9 & 12 &   c & 478 & 9 & 12 &    \\
e & 12 & 191 & 7 &   e & 12 & 191 & 7 & \\
o & 22 & 6 & 72 &   o & 22 & 6 & 72 &  \\ \cmidrule(r){1-4} \cmidrule(lr){5-8} 
\end{tabular}

\\

\begin{tabular}{@{}lrrrrrrrrr@{}}
\cmidrule(r){1-4} \cmidrule(lr){5-8} 
\begin{tabular}[c]{@{}l@{}}\textcolor{red}{DT} LDA\\ max SDS-score\end{tabular} & c & e & o &   \begin{tabular}[c]{@{}l@{}}\textcolor{red}{DT} LDA\\ max F-measure\end{tabular} & c & e & o &\\ \cmidrule(r){1-4} \cmidrule(lr){5-8} 
c & 482 & 9 & 8 &   c & 482 & 9 & 8 &    \\
e & 17 & 187 & 6 &   e & 17 & 187 & 6 & \\
o & 21 & 7 & 72 &   o & 21 & 7 & 72 &  \\ \cmidrule(r){1-4} \cmidrule(lr){5-8} 
\end{tabular}
%}
%\caption{Fine-tuned DT and RF confusion matrices comparison with PCA}
\label{confusion_rf_3}

\\

\begin{tabular}{@{}lrrrrrrrrr@{}}
\cmidrule(r){1-4} \cmidrule(lr){5-8} 
\begin{tabular}[c]{@{}l@{}}SVM \textcolor{red}{15 features}\\ max SDS-score\end{tabular} & c & e & o &   \begin{tabular}[c]{@{}l@{}}SVM \textcolor{red}{15 featuresn}\\ F-measure\end{tabular} & c & e & o &\\ \cmidrule(r){1-4} \cmidrule(lr){5-8} 
c & 490 & 6 & 3 &   c & 490 & 6 & 3 &    \\
e & 9 & 195 & 6 &   e & 9 & 195 & 6 & \\
o & 25 & 5 & 237 &   o & 25 & 5 & 237 &  \\ \cmidrule(r){1-4} \cmidrule(lr){5-8} 
\end{tabular}%

\\

\begin{tabular}{@{}lrrrrrrrrr@{}}
\cmidrule(r){1-4} \cmidrule(lr){5-8} 
\begin{tabular}[c]{@{}l@{}}DT \textcolor{red}{15 features}\\ max SDS-score\end{tabular} & c & e & o &   \begin{tabular}[c]{@{}l@{}}DT \textcolor{red}{15 features}\\ max F-measure\end{tabular} & c & e & o &\\ \cmidrule(r){1-4} \cmidrule(lr){5-8} 
c & 490 & 5 & 4 &   c & 490 & 5 & 4 &    \\
e & 8 & 197 & 5 &   e & 8 & 197 & 5 & \\
o & 26 & 10 & 64 &   o & 26 & 10 & 64 &  \\ \cmidrule(r){1-4} \cmidrule(lr){5-8} 
\end{tabular}%

\\

\begin{tabular}{@{}lrrrrrrrrr@{}}
\cmidrule(r){1-4} \cmidrule(lr){5-8} 
\begin{tabular}[c]{@{}l@{}}RF \textcolor{red}{15 features}\\ SDS-score\end{tabular} & c & e & o &   \begin{tabular}[c]{@{}l@{}}RF \textcolor{red}{15 features}\\ F-measure\end{tabular} & c & e & o &\\ \cmidrule(r){1-4} \cmidrule(lr){5-8} 
c & 488 & 7 & 4 &   c & 489 & 7 & 3 &    \\
e & 7 & 194 & 9 &   e & 8 & 194 & 8 & \\
o & 22 & 4 & 74 &   o & 22 & 3 & 75 &  \\ \cmidrule(r){1-4} \cmidrule(lr){5-8} 
\end{tabular}%
%\caption{SVM confusion matrices comparison}
\label{confusion_rf_4}

\\

\begin{tabular}{@{}lrrrrrrrrr@{}}
\cmidrule(r){1-4} \cmidrule(lr){5-8} 
\begin{tabular}[c]{@{}l@{}}ET \textcolor{red}{15 features}\\ SDS-score\end{tabular} & c & e & o &   \begin{tabular}[c]{@{}l@{}}ET \textcolor{red}{15 features}\\ F-measure\end{tabular} & c & e & o &\\ \cmidrule(r){1-4} \cmidrule(lr){5-8} 
c & 487 & 8 & 4 &   c & 487 & 8 & 4 &    \\
e & 7 & 198 & 5 &   e & 7 & 198 & 5 & \\
o & 27 & 5 & 68 &   o & 27 & 5 & 68 &  \\ \cmidrule(r){1-4} \cmidrule(lr){5-8} 
\end{tabular}%
%\caption{Gradient booster confusion matrices comparison}
\label{confusion_et_2}
%end{table*}

\\

\begin{tabular}{@{}lrrrrrrrrr@{}}
\cmidrule(r){1-4} \cmidrule(lr){5-8} 
\begin{tabular}[c]{@{}l@{}}GB \textcolor{red}{15 features}\\ SDS-score\end{tabular} & c & e & o &   \begin{tabular}[c]{@{}l@{}}GB \textcolor{red}{15 features}\\ F-measure\end{tabular} & c & e & o &\\ \cmidrule(r){1-4} \cmidrule(lr){5-8} 
c & 488 & 6 & 5 &   c & 488 & 6 & 5 &    \\
e & 8 & 194 & 8 &   e & 8 & 194 & 8 & \\
o & 20 & 5 & 75 &   o & 20 & 5 & 75 &  \\ \cmidrule(r){1-4} \cmidrule(lr){5-8} 
\end{tabular}%
%\caption{Random forest confusion matrices comparison}
\label{confusion_gb_5}

\\

\begin{tabular}{@{}lrrrrrrrrr@{}}
\cmidrule(r){1-4} \cmidrule(lr){5-8} 
\begin{tabular}[c]{@{}l@{}}kNN \textcolor{red}{15 features}\\ SDS-score\end{tabular} & c & e & o &   \begin{tabular}[c]{@{}l@{}}kNN \textcolor{red}{15 featuresn}\\ F-measure\end{tabular} & c & e & o &\\ \cmidrule(r){1-4} \cmidrule(lr){5-8} 
c & 489 & 8 & 2 &   c & 489 & 8 & 2 &    \\
e & 12 & 193 & 5 &   e & 12 & 193 & 5 & \\
o & 30 & 7 & 63 &   o & 30 & 7 & 63 &  \\ \cmidrule(r){1-4} \cmidrule(lr){5-8} 
\end{tabular}%
%\caption{Extra trees confusion matrices comparison}
\label{confusion_knn_2}

\\

\begin{tabular}{@{}lrrrrrrrrr@{}}
\cmidrule(r){1-4} \cmidrule(lr){5-8} 
\begin{tabular}[c]{@{}l@{}}MLP \textcolor{red}{15 features}\\ SDS-score\end{tabular} & c & e & o &   \begin{tabular}[c]{@{}l@{}}MLP \textcolor{red}{15 featuresn}\\ F-measure\end{tabular} & c & e & o &\\ \cmidrule(r){1-4} \cmidrule(lr){5-8} 
c & 485 & 6 & 8 &   c & 485 & 6 & 8 &    \\
e & 9 & 194 & 7 &   e & 9 & 194 & 7 & \\
o & 19 & 5 & 76 &   o & 19 & 5 & 76 &  \\ \cmidrule(r){1-4} \cmidrule(lr){5-8} 
\end{tabular}%
\\
\caption{Confusion matrices for the second experiment (raw data Table~\ref{tab:best_experiment_lda}).}
\label{confusion_table_resum_2}
\end{longtable}
